# Supplementary material for: Dynamic Sequential Graph Learning for Click-Through Rate Prediction
Source: arXiv:2109.12541 source file (2021-09-26)
Supplement: Supplementary file 1 [file 6_appendix.tex]

\clearpage

\section{Reproducibility Details}
We have omitted some details in the main paper and present them here for reproducibility. We first describe the datasets in more details including the statistics and the preprocessing. Then additional implementation notes and the experimental environment are presented. Finally, we give detailed implementation notes of baselines.

\subsection{Dataset Statistics and Preprocessing}\label{apendix:data}
The statistics of each dataset are shown in Table \ref{data}.
We performed a temporal train-test split, i.e., dividing the dataset into training and testing dataset by a cut timestamp, with the first 85\% for training and the rest 15\% for testing. For all methods, we conduct the negative sampling strategy to pair each user with one negative item that the user does not interact with. 

To construct dynamic sequential graphs, we first build the user behavior sequence and item behavior sequence ordered by the interaction time for each user-item sample in the dataset. We truncate the sequence by selecting the last $m$ elements to align the sequence lengths among samples. For each interaction $(u,i,t)$, with the behavior sequence $\gS_{u,t}$ before time $t$ of the user $u$, we can build a dictionary $\{(u,t):\gS_{u,t}\}$ with tuple $(u,t)$ as the key and $\gS_{u,t}$ as the value. $\gS_{u,t}$ can be seen as the child nodes of the 1-depth DSG and stored in a list. Similarly, we can obtain the dictionary $\{(i,t):\gS_{i,t}\}$ for item $i$. By join the two dictionaries, we can obtain the nested dictionaries $\{(u,t):\{(i,\tau):\gS_{i,\tau}\}\}$ and $\{(i,t):\{(u,\tau):\gS_{u,\tau}\}\}$, and they can be seen as the 2-depth DSGs. By analogy, we can get the $K$-layer DSGs recursively. Each layer of nodes with the interaction time can be stored in Tensors with the shape of $(B,m^1,\dots,m^K,2)$, where $B$ denotes the mini-batch size and $m^k$ is the truncation length of $k$-th layer.
\begin{table}[ht]
\centering
\setlength\abovecaptionskip{2pt}
\caption{Hyper-parameter Settings of DSGL.}
% \resizebox{\linewidth}{!}{
\begin{tabular}{@{}l|l@{}}
\toprule
Hyper-parameter & Setting \\ \midrule
    Learning rate   &   0.001 \\
    Optimizer & Adam \\
    Initializer of embedding parameters & Xavier uniform initializer\\
    Mini-batch size & 128 \\
    User ID embedding dimension  & 64 \\
    Item ID embedding dimension  & 32 \\
    Category ID embedding dimension  & 32 \\
    Time decay feature dimension  & 32 \\
    \makecell[l]{Hidden units of the time-aware \\ sequence encoding}  & 64 \\
    \makecell[l]{Hidden units of the second-order \\ graph attention}  & 64 \\
    \makecell[l]{Hidden units of the prediction layer} & \{256,128\} \\
    Number of layers & 3 \\
    \makecell[l]{Number of neighbors at each layer \\of the DSG of the target users} & \{100,5,5\} \\
    \makecell[l]{Number of neighbors at each layer \\of the DSG of the candidate items} & \{50,5\} \\
    \makecell[l]{Number of attention heads} & 4 \\
    \makecell[l]{Base of time bucket bounds} & 2 \\
    \bottomrule
\end{tabular}
\label{tab:hyp}
% }
\end{table}

\begin{table}[ht]
\centering
\setlength\abovecaptionskip{2pt}
\caption{Hyper-parameter Settings of Baselines.}
\resizebox{\linewidth}{!}{
\begin{tabular}{@{}l|l@{}}
\toprule
\multicolumn{2}{c}{Shared Settings (same as DSGL)}\\ \midrule
Prediction loss & the cross-entropy loss \\
    Learning rate   &   0.001 \\
    Optimizer & Adam \\
    Initializer of embedding parameters & Xavier uniform initializer\\
    Mini-batch size & 128 \\
    User ID embedding dimension  & 64 \\
    Item ID embedding dimension  & 32 \\
    Category ID embedding dimension  & 32 \\
    Time decay feature dimension  & 32 \\
    User behavior sequence length (if utilize)  & 100 \\
    Item behavior sequence length (if utilize)  & 50 \\
    \makecell[l]{Hidden units of the prediction layer} & \{256,128\} \\ \toprule
    \multicolumn{2}{c}{GRU4Rec, Topo-LSTM, DIB, TIEN} \\ \midrule
    Hidden units in GRU layers & \{64,64\}\\ \toprule
    \multicolumn{2}{c}{DIN} \\ \midrule
    Hidden units in DIN attention & \{80,40\} \\ \toprule
    \multicolumn{2}{c}{DIB} \\ \midrule
    \makecell[l]{Number of dynamic item block factors}  & 32 \\\toprule
    \multicolumn{2}{c}{LightGCN, NGCF} \\ \midrule
    \makecell[l]{GNN layers}  & 3 \\\bottomrule
\end{tabular}
\label{tab:hypbase}
}
\end{table}

% \subsection{Additional Implementation Notes}
\subsection{Additional Implementation Notes}
Table~\ref{tab:hyp} is the hyper-parameter setting of our method, and we use the same hyper-parameters for all datasets to ensure the fairness of the comparison. 

For DSGL and all the baselines, the early stopping strategy is performed, i.e., terminate training if AUC on the validation data does not increase for 10 successive iterations. We save the checkpoints every 100 steps, and choose the checkpoint with best AUC among these checkpoints as the final model.

% The performance is evaluated through the metric AUC and Logloss
% , whose definitions are as follows:
% \begin{equation}
%     \text{AP} = \sum_n (R_n - R_{n-1}) P_n
% \end{equation}
In the experiments, the final metrics are implemented by Scikit-learn\footnote{https://scikit-learn.org/} tool with the functions  \texttt{sklearn.metrics.roc\_auc\_score} for AUC and \texttt{sklearn.metrics.log\_loss} for Logloss.

\subsection{Experiment Environment}
All experiments are conducted on a server with one GPU (GeForce GTX 1080 Ti), and implemented with the TensorFlow Estimator API. The versions of Python and TensorFlow are 2.7 and 1.12, respectively.

\subsection{Implementation of Baselines}\label{apendix:baseline}
We classify the compared methods into the following five categories:
\begin{itemize}[leftmargin=10pt]
    \item \textbf{Conventional methods:}
    \begin{itemize}
        % \item \textbf{YoutubeDNN} gets user representations by simply averaging the item embeddings in the user behavior sequence.
        \item \textbf{SVD++}~\cite{koren2008factorization} is a hybrid method of latent factor model and neighbor based model. 
        \item \textbf{PNN}~\cite{qu2016product} uses a product layer to capture high-order feature interactions between interfield categories
    \end{itemize}
    \item \textbf{Sequential methods with user behaviors:}
        \begin{itemize}
        \item \textbf{GRU4Rec}~\cite{hidasi2015session} is the first RNN-based method which simply stacks multiple GRU layers to model users' historical behavior sequences for recommendation. 
        \item \textbf{CASER}~\cite{tang2018personalized} is a CNN-based sequential recommendation method, which models the union-level sequential patterns by capturing local sequential patterns of adjacent items.
        \item \textbf{ATRANK}~\cite{zhou2018atrank} is an attention-based framework to model the user behavior sequence.
        \item \textbf{DIN}~\cite{zhou2018deep} uses the attention mechanism to activate related user behaviors.
        % \item \textbf{DIEN}~\cite{zhou2019deep} uses GRU with attentional update gate to model users' dynamic interest that is relative to the candidate item.
    \end{itemize}
    \item \textbf{Sequential methods with user and item behaviors:}
        \begin{itemize}
        \item \textbf{Topo-LSTM}~\cite{wang2017topological} uses LSTM to model both user and item behavior sequences to capture their dynamics.
        \item \textbf{DIB}~\cite{guo2019dynamic} learns dynamic item representation by aggregating users in item behaviors most similar to target users.
        \item \textbf{TIEN}~\cite{li2020deep} leverages GRU with attention mechanism to capture both time-aware user behaviors and item behaviors.
    \end{itemize}
    \item \textbf{Static-graph-based methods:}
    \begin{itemize}
        \item \textbf{NGCF}~\cite{wang2019neural} is a GCN-based collaborative filtering method. It explicitly integrates a bipartite graph structure into the embedding learning process to model the high-order connectivity in the user-item graph.
        \item \textbf{LightGCN}~\cite{he2020lightgcn} is the state-of-the-art GCN-based collaborative filtering method, which simplifies the design of GCN to make it appropriate for recommendation by light graph convolution and layer combination.
    \end{itemize}
    \item \textbf{Dynamic-graph-based methods:}
    \begin{itemize}
        \item \textbf{SR-GNN}~\cite{wu2019session} models each session sequence a directed graph, capturing the complex structure and transitions between items of session sequences.
    \end{itemize}
\end{itemize}
The hyper-parameters of these baselines are listed in Table~\ref{tab:hypbase}.
